# Supplementary material for: Benchmarking VLMs' Reasoning About Persuasive Atypical Images
Source: arXiv:2409.10719 source file (2024-12-16)
Supplement: Supplementary file 2 [file supp_tab_gpt4v_complete.tex]

\setlength{\tabcolsep}{1pt}
\begin{table}[!htp]\centering
\caption{GPT4-V experiments}\label{tab:supp_gpt4v_results}
\scriptsize
\begin{tabular}{lc||ccc||c||ccc|ccc||c}\toprule
\multirow{3}{*}{\textbf{Classifier}}& \multirow{3}{*}{\textbf{Method}}& \multicolumn{3}{c||}{\textbf{\textit{MAC}}}& \textbf{\textit{ASR}} &\multicolumn{6}{c||}{\textbf{\textit{ARR multi}}}  & \textbf{\textit{ARR Single}}\\

& & \multirow{2}{*}{\textbf{precision}} & \multirow{2}{*}{\textbf{recall}} & \multirow{2}{*}{\textbf{f1-score}} &Acc& \multicolumn{3}{c}{\textbf{precision@k}} & \multicolumn{3}{c||}{\textbf{Top-k acc}}&\multirow{2}{*}{\textbf{Acc}} \\
 & & & & & &\textbf{k=1} &\textbf{k=2 }&\textbf{k=3} &\textbf{k=1} &\textbf{k=2} &\textbf{k=3} \\
\hline
\hline
LLaVA &- &0 &0 &0 &0 &0 &0 &0 &0 &0 &0 &0 \\
GPT4-V &- &0 &0 &0 &0 &0 &0 &0 &0 &0 &0&0 \\
GPT-4 &$\mathcal{T}_\mathcal{V}$ &0 &0 &0 &0 &0 &0 &0 &0 &0 &0 &0\\
GPT-4 & $\mathcal{T}_\mathcal{V} + \hat{s}_{IN}$ &0 &0 &0 &0 &0 &0 &0 &0 &0 &0 &0 \\
\bottomrule
\end{tabular}
\end{table}
